# Supplementary material for: Absence of magnetic order and emergence of unconventional fluctuations in $J_{\rm eff} =1/2$ triangular lattice antiferromagnet YbBO$_3$
Source: arXiv:2210.09724 source file (2022-10-18)
Supplement: Supplementary file 1 [file SM.pdf]

# Supplementary Material for "Absence of magnetic order and emergence of unconventional fluctuations in $J_{\text{eff}} = 1/2$ triangular lattice antiferromagnet $\text{YbBO}_3$ "

K. Somesh,<sup>1</sup> S. S. Islam,<sup>1</sup> S. Mohanty,<sup>1</sup> G. Simutis,<sup>2,3,\*</sup> Z. Guguchia,<sup>4</sup> Ch.  
Wang,<sup>4</sup> R. Scheuermann,<sup>4</sup> J. Sichelschmidt,<sup>5</sup> M. Baenitz,<sup>5</sup> and R. Nath<sup>1,†</sup>

<sup>1</sup>*School of Physics, Indian Institute of Science Education and Research Thiruvananthapuram-695551, India*

<sup>2</sup>*Laboratory for Neutron and Muon Instrumentation,  
Paul Scherrer Institut, CH-5232 Villigen PSI, Switzerland*

<sup>3</sup>*Department of Physics, Chalmers University of Technology, SE-41296 Göteborg, Sweden*

<sup>4</sup>*Laboratory for Muon Spin Spectroscopy, Paul Scherrer Institut, Villigen PSI, Switzerland*

<sup>5</sup>*Max Planck Institute for Chemical Physics of Solids,  
Nöthnitzer Strasse 40, 01187 Dresden, Germany*

(Dated: September 27, 2022)

Polycrystalline sample of  $\text{YbBO}_3$  was synthesized by solid-state technique. The stoichiometric mixture of high purity reagents  $\text{Yb}_2\text{O}_3$  and  $\text{H}_3\text{BO}_3$  (15% excess to compensate the loss of B during the heating process due to volatile nature of  $\text{H}_3\text{BO}_3$ ) were grounded and preheated at  $500^\circ\text{C}$  to decompose  $\text{H}_3\text{BO}_3$  to  $\text{B}_2\text{O}_3$  followed by a firing at  $900^\circ\text{C}$  with intermediate grinding. The phase purity of the sample was confirmed by the powder x-ray diffraction (XRD) measurement using a PANalytical x-ray diffractometer ( $\text{Cu } K_\alpha$  radiation,  $\lambda_{\text{av}} = 1.54182 \text{ \AA}$ ). The temperature-dependent powder XRD measurements were performed over the temperature range  $15 \text{ K} \leq T \leq 300 \text{ K}$  using a low temperature attachment (Oxford Phenix) to the diffractometer. Magnetization ( $M$ ) measurements were performed as a function of temperature ( $T$ ) and applied field ( $H$ ) using a superconducting quantum interference device (SQUID) (MPMS-3, Quantum Design). Measurements down to  $0.4 \text{ K}$  were carried out using a  $^3\text{He}$  (iHelium3, Quantum Design Japan) attachment to the MPMS. Heat capacity [ $C_p(T)$ ] measurements were performed on a small piece of sintered pellet using the relaxation technique in the physical property measurement system (PPMS, Quantum Design). For measurements down to  $0.4 \text{ K}$ ,  $^3\text{He}$  attachment was used to the PPMS.

We investigated the Electron Spin Resonance (ESR) of polycrystalline  $\text{YbBO}_3$  using a standard continuous-wave ESR setup at X-band frequency ( $9.4 \text{ GHz}$ ). The temperature was varied between  $3$  and  $295 \text{ K}$  with a He-flow cryostat. ESR can be detected by the absorbed power  $P$  of a transversal magnetic microwave field as a function of a static, external magnetic field  $\mu_0 H$ . To improve the signal-to-noise ratio, we used a lock-in technique by modulating the static field, which yields the derivative of the resonance signal  $dP/dH$ . The measured ESR spectra were fitted with a Lorentzian function including the influence of the counter-rotating component of the linearly polarized microwave field [S1]. From the fit we obtained the linewidth  $\Delta H$  and the resonance field  $H_{\text{res}}$  which determines the ESR  $g$ -factor  $g = h\nu/\mu_B H_{\text{res}}$ . The ESR intensity  $I_{\text{ESR}}$  is a measure of the local static susceptibility of the probed ESR spin, i.e. in our case the local susceptibility of the  $\text{Yb}^{3+}$  spins [S2]. We calculated  $I_{\text{ESR}} \approx \text{Amp} \cdot \Delta H^2$  which approximates the integrated ESR absorption [S3].

The muon spin relaxation ( $\mu\text{SR}$ ) measurements were performed at the  $S\mu\text{S}$  muon source at Paul Scherrer Institute using a combination of two spectrometers. The high temperature measurements ( $1.5 \text{ K} - 50 \text{ K}$ ) were performed using low-background high-throughput instrument GPS [S4]. The low temperature data points were acquired using the zero field option of the HAL spectrometer which allowed reaching temperatures as low as  $20 \text{ mK}$ . An overlapping temperature region was studied in both spectrometers to account for different sample holders and the fact that for the HAL measurement a pellet was made out of powder and mixed with GE-vanish for structural stability and to ensure the thermal contact.

## X-RAY DIFFRACTION

$\text{YbBO}_3$  belongs to the family having the general formula  $RE\text{BO}_3$  ( $RE = \text{rare-earth}$ ) with the hexagonal crystal system of space group  $P6_3/m$  (No. 176) [S5]. The crystal structure is constituted with lanthanide ions which is coordinated to eight oxygen atoms forming a trigonal bipyramidal antiprism. Figure 1(a) of main text shows the crystal structure of  $\text{YbBO}_3$  containing the triangular layers of  $\text{Yb}^{3+}$  ions with interlayer spacing of  $4.395 \text{ \AA}$ , which is separated by layers of three-membered rings of  $(\text{BO}_4)^{5-}$  units. Figure 1(b) presents the in-plane structure of the  $\text{Yb}^{3+}$  forming a triangular units with nearest neighbor (NN) distance  $3.751 \text{ \AA}$ . The ratio of inter-plane to in-plane distance ( $d_{\text{inter}}/d_{\text{intra}}$ ) between  $\text{Yb}^{3+}$  ions is  $1.17$ .

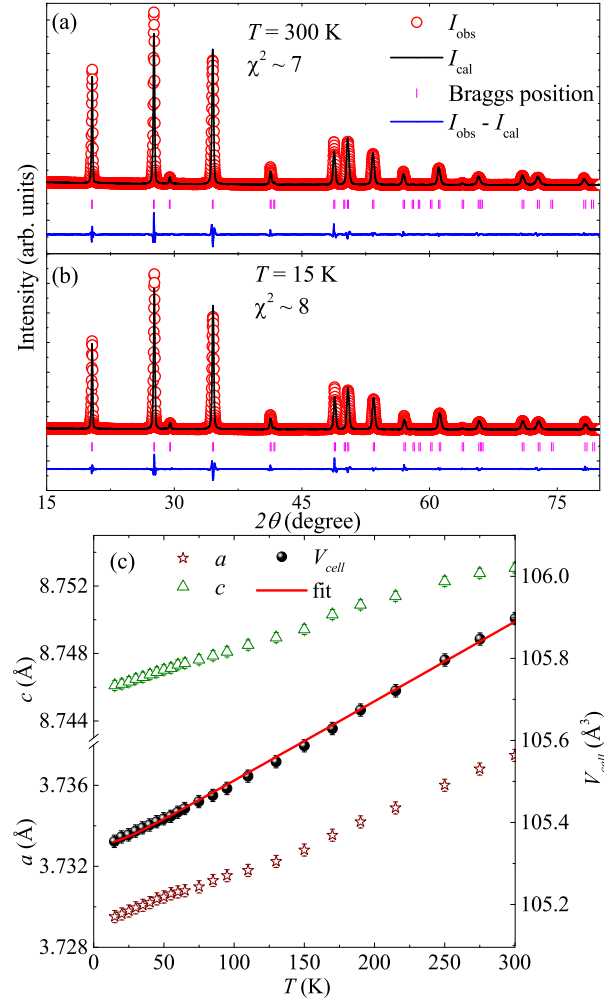

FIG. S1. Powder XRD data measured at (a)  $T = 300$  K and (b)  $T = 15$  K. The red solid line represents the Rietveld fit of the data. Bragg positions are indicated by pink vertical bars and the solid blue line at the bottom denotes the difference between experimental and calculated intensities. (c) The variation of lattice parameters ( $a$ ,  $c$ , and  $V_{cell}$ ) as a function of temperature. The solid line denotes the fit of  $V_{cell}(T)$  by Eq. (S1).

In order to confirm the phase purity of the sample, powder XRD data were collected at various temperatures. Rietveld refinement of the XRD data were carried out using FullProf software package, confirming the formation of pure phase with neither a structural distortion nor a phase transition observed down to 15 K shown in Fig. S1(a) and (b). All peaks in the XRD data appropriately indexed to the space group  $P6_3/m$  (No. 176) with the obtained lattice parameters at room temperature as  $a = b = 3.7344(1)$  Å,  $c = 8.7433(1)$  Å, and  $V_{cell} \simeq 105.59(1)$ , which are fairly comparable with the previous report [S5]. The atomic coordinates of the different elements after the refinement are shown in Table S1. Figure S1(c) presents the variation of lattice parameters over the temperature range 15 K to 300 K. Upon cooling to 15 K, the parameters decrease monotonically. The temperature variation of  $V_{cell}$  was fitted by the equation [S6]

$$V(T) = \gamma U(T)/K_0 + V_0, \quad (S1)$$

where  $V_0$  is the cell volume at  $T = 0$  K,  $K_0$  is the bulk modulus, and  $\gamma$  is the Grüneisen parameter.  $U(T)$  is the internal energy which can be derived in terms of the Debye approximation as,

$$U(T) = 9nk_B T \left( \frac{T}{\theta_D} \right)^3 \int_0^{\theta_D/T} \frac{x^3}{e^x - 1} dx. \quad (S2)$$

Here,  $n$  is the number of atoms in the unit cell and  $k_B$  is the Boltzmann constant. Using this approximation

TABLE S1. Listed are the Wyckoff positions and the refined atomic coordinates ( $x$ ,  $y$ , and  $z$ ) for each atom at room temperature.

| Atom | Site | $x$      | $y$       | $z$      | Occupancy |
|------|------|----------|-----------|----------|-----------|
| O1   | 4f   | 0.667    | 0.333     | 0.107(7) | 1         |
| O2   | 6h   | 0.776(5) | -0.197(6) | 0.25     | 0.333     |
| B1   | 6h   | 0.575(7) | 0.417(8)  | 0.25     | 0.333     |
| Yb1  | 2b   | 0        | 0         | 0        | 1         |

(see Fig. S1(c)), the Debye temperature ( $\theta_D$ ) and other parameters were estimated to be  $\theta_D \simeq 208$  K,  $\gamma/K \simeq 1.83 \times 10^{-5}$  Pa $^{-1}$ , and  $V_0 \simeq 105.384$  Å $^3$ .

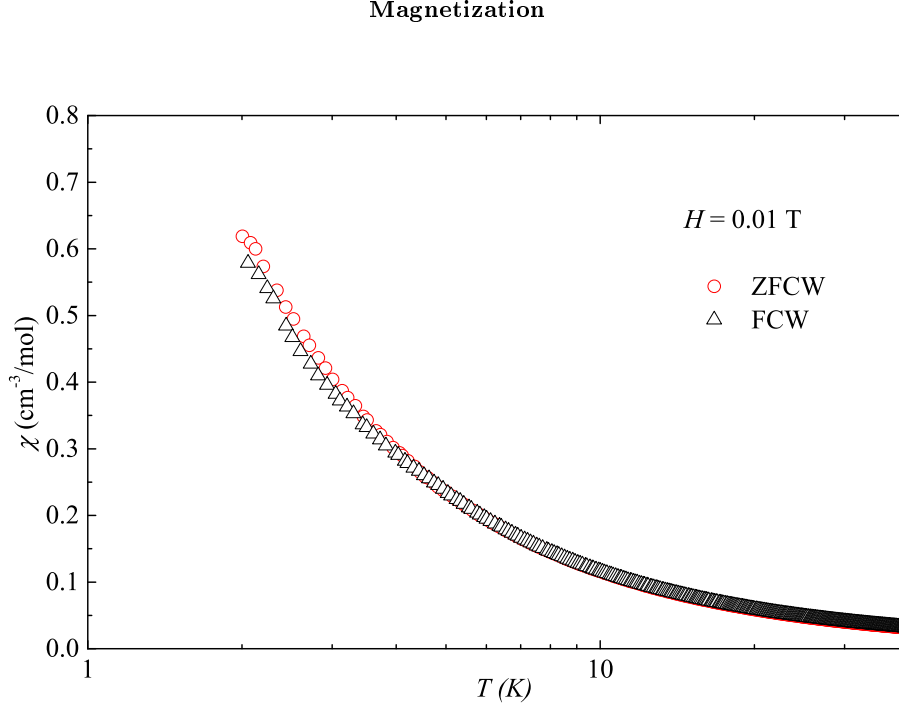FIG. S2. Absence of bifurcation pictured in the plot of  $\chi$  vs  $T$  between ZFC and FC data at  $H = 100$  Oe.

Figure S2 presents the measurements in zero field cooled (ZFC) and field cooled (FC) protocols. The absence of bifurcation between ZFC and FC data rules out spin freezing or a spin glass transition down to  $T = 2$  K.

The magnetic isotherm measured at  $T = 0.4$  K along with the linear fit indicating the Van-Vleck contribution is presented in Fig. S3. One can estimate  $\chi_{VV}$  and  $M_{\text{sat}}$  from slope and intercept of the fit, respectively. The fit yields  $\chi_{VV} \simeq 3.32 \times 10^{-3}$  cm $^3$ /mol and  $M_{\text{sat}} \simeq 8892.2$  G.cm $^3$ /mol =  $1.6 \mu_B$ .

### ELECTRON SPIN RESONANCE

Electron spin resonance (ESR) signals for three typical temperature regimes are shown in the Fig. S4(a). The most well-defined spectral shapes were detected in a temperature regime between 20 K and 80 K with a corresponding  $g$ -value of  $g = 3.4(0)$  as indicated by the red solid Lorentzian line shape. The low temperature Curie-Weiss (CW) fit of  $I_{\text{ESR}}^{-1}$  [presented in Fig. S4(c)] yields a small CW temperature ( $\theta_{\text{CW}}$ ) of  $\sim -1$  K is consistent with the uncertainties in the determination of  $I_{\text{ESR}}$ . The temperature dependence of the linewidth is shown in Fig. S4(b). For temperatures above  $\sim 70$  K the ESR linewidth broadens according to  $\Delta H \propto 1/\exp(\Delta_{\text{ESR}}/k_B T) - 1$ , see the red solid line. This behavior indicates a spin-lattice relaxation dominated by an Orbach process. Via spin-orbit coupling this process involves a phonon absorption to and emission from a crystalline-electric field split electronic energy level  $\Delta_{\text{ESR}}$  above

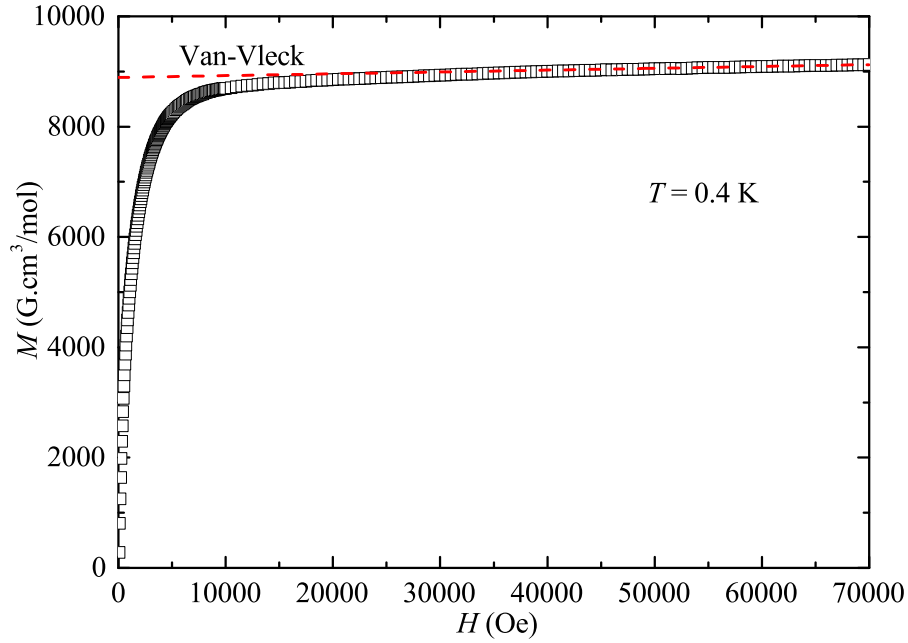

FIG. S3. Magnetic isotherm measured at 0.4 K. The red dashed line represents the Van-Vleck contribution.

the ground state [S2, S7]. We obtained  $\Delta_{\text{ESR}}/k_{\text{B}} = (500 \pm 100)$  K. Towards low temperatures the spectra display a moderate broadening, indicating the increasing influence of  $\text{Yb}^{3+}$  spin correlations.

- 
- [S1] D. Rauch, M. Kraken, F. J. Litterst, S. Süllow, H. Luetkens, M. Brando, T. Förster, J. Sichelschmidt, A. Neubauer, C. Pfeiderer, W. J. Duncan, and F. M. Grosche, Spectroscopic study of metallic magnetism in single-crystalline  $\text{Nb}_{1-y}\text{Fe}_{2+y}$ , *Phys. Rev. B* **91**, 174404 (2015).
  - [S2] A. Abragam and B. Bleaney, *Electron paramagnetic resonance of transition ions* (OUP Oxford, 2012).
  - [S3] K. M. Ranjith, D. Dmytriieva, S. Khim, J. Sichelschmidt, S. Luther, D. Ehlers, H. Yasuoka, J. Wosnitzer, A. A. Tsirlin, H. Kühne, and M. Baenitz, Field-induced instability of the quantum spin liquid ground state in the  $J_{\text{eff}} = \frac{1}{2}$  triangular-lattice compound  $\text{NaYbO}_2$ , *Phys. Rev. B* **99**, 180401 (2019).
  - [S4] A. Amato, H. Luetkens, K. Sedlak, A. Stoykov, R. Scheuermann, M. Elender, A. Raselli, and D. Graf, The new versatile general purpose surface-muon instrument (GPS) based on silicon photomultipliers for  $\mu^+$ SR measurements on a continuous-wave beam, *Rev. Sci. Instrum.* **88**, 093301 (2017).
  - [S5] G. Chadeyron, M. El-Ghozzi, R. Mahiou, A. Arbus, and J. Cousseins, Revised Structure of the Orthoborate  $\text{YBO}_3$ , *J. Solid State Chem.* **128**, 261 (1997).
  - [S6] K. Somesh, Y. Furukawa, G. Simutis, F. Bert, M. Prinz-Zwick, N. Büttgen, A. Zorko, A. A. Tsirlin, P. Mendels, and R. Nath, Universal fluctuating regime in triangular chromate antiferromagnets, *Phys. Rev. B* **104**, 104422 (2021).
  - [S7] R. . Orbach and B. Bleaney, Spin-lattice relaxation in rare-earth salts, *Proc. Math. Phys. Eng. Sci.* **264**, 458 (1961)

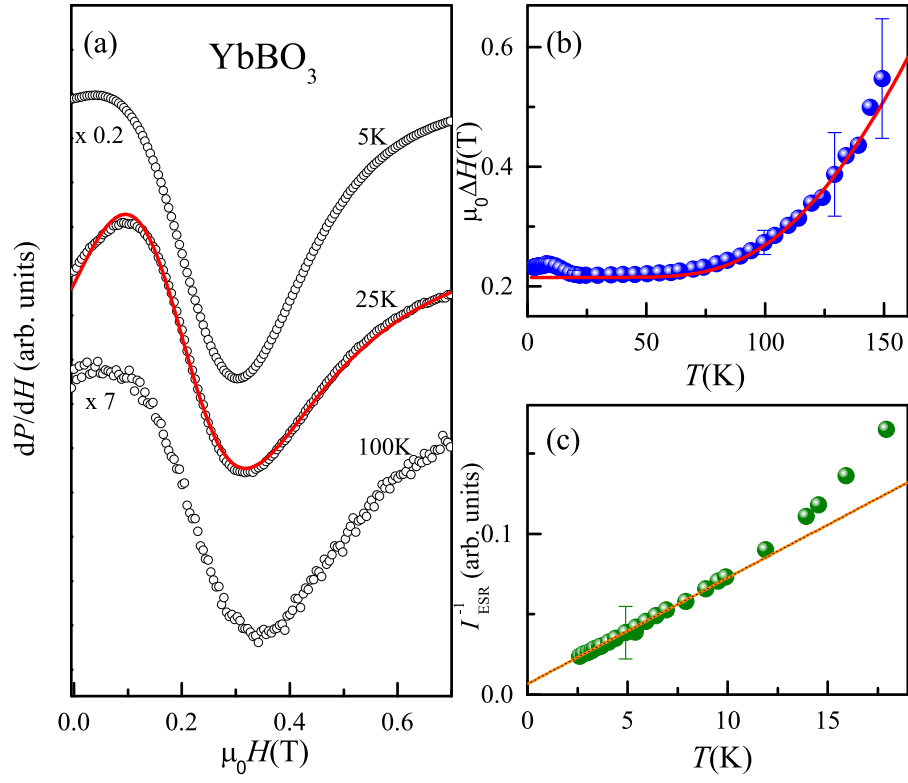

FIG. S4. (a) Electron spin resonance spectra of  $\text{YbBO}_3$  at temperatures and with magnifications as indicated. The red solid line depicts a Lorentzian line shape with a  $g$ -value of  $g = 3.4(0)$ . (b) The ESR linewidth  $\Delta H$  where the solid line refers at higher temperatures to a relaxation mechanism via the first excited crystalline electric field level of  $\text{Yb}^{3+}$  at  $\Delta_{\text{ESR}}/k_B = (500 \pm 100)$  K. (c) Temperature dependence of the reciprocal ESR intensity  $I_{\text{ESR}}^{-1}$  (solid lines suggest linear behavior).
